# Supplementary material for: Low-Mass Dark Matter Search with CDMSlite
Source: arXiv:1707.01632 ancillary file (2018-01-18)
Supplement: Supplementary file 1 [file CDMSlite_Run2_DataRelease_Document.pdf]

# CDMSlite Run 2 Data Release

SuperCDMS Collaboration

January 17, 2018

This document accompanies the public release of the CDMSlite Run 2 data and gives explanatory material related to the released files themselves and their use in reproducing published upper limit results. The WIMP-search results from these data are found in the articles arXiv:1509.02448 [1] and arXiv:1707.01632 [2]. The released data and code have been internally verified to reproduce the official limits and figures presented in this release document. Questions about the data or the limits should be directed to `supercdms_publications@lists.astro.caltech.edu`.

The published upper limits on WIMP-nucleon interactions were computed by sampling the uncertainties associated with the analysis. This was accomplished by creating 1000 realizations of the analysis, where each realization was the result of a single sampling of the uncertainty distributions. An upper limit was then computed with each realization to generate a distribution 1000 limits. The official limits and uncertainties were then taken as the medians and central 95 % intervals from the limit distributions. The methodology and data necessary to duplicate this procedure are discussed below and included in this release. However, given the burden to recreate this procedure, an alternative limit setting procedure is discussed and provided. This alternative is termed the “best-fit” method<sup>1</sup> which computes a single limit per interaction. For all instances below, both of these methods of limit setting are discussed.

## 1 Energy Scales in CDMSlite

The total phonon signal  $E_t$  measured by the CDMSlite detector is given by the sum of the initial recoil  $E_r$  and Neganov-Trofimov-Luke  $E_{\text{NTL}} = E_r Y(E_r) e V_b / \epsilon_\gamma$  phonons [3, 4]

$$E_t = E_r \left( 1 + Y(E_r) \frac{e V_b}{\epsilon_\gamma} \right), \quad (1)$$

where  $e$  is the elementary charge,  $V_b = 70$  V is the applied potential difference,  $\epsilon_\gamma = 3$  eV/pair is the average energy required to create an electron-hole pair for an electron recoil (ER) in germanium [5], and  $Y(E_r)$  is the recoil-energy, and recoil-type, dependent ionization yield. Events are either electron recoils with  $Y(E_r) \equiv 1$  or nuclear recoils (NRs) with  $Y(E_r) < 1$ . The CDMSlite measurement technique cannot directly measure  $Y(E_r)$  and therefore cannot

---

<sup>1</sup>Note that the label “best-fit” is applied loosely here, as it is not the result of a fitting procedure. See below.

know the recoil type on an event-by-event basis. Instead, the measured energy spectrum is first calibrated assuming all events are ERs. This energy scale is termed “electron-equivalent” and denoted by units of  $\text{keV}_{\text{ee}}$ . A model for  $Y(E_r)$  is then employed to convert all events to the NR-energy scale termed “nuclear-recoil-equivalent” and denoted by units of  $\text{keV}_{\text{nr}}$ . The data included in this release are in  $\text{keV}_{\text{ee}}$  units with the conversion to  $\text{keV}_{\text{nr}}$  left to the user to allow for freedom of choice in ionization yield models.

The model used in the published analysis is that of Lindhard [6]

$$Y(E_{\text{nr}}) = \frac{k \cdot g(\varepsilon)}{1 + k \cdot g(\varepsilon)}, \quad (2)$$

where  $g(\varepsilon) = 3\varepsilon^{0.15} + 0.7\varepsilon^{0.6} + \varepsilon$ ,  $\varepsilon = 11.5E_{\text{nr}}(\text{keV})Z^{-7/3}$ , and  $Z$  is the atomic number of the material. For germanium, the standard value is  $k = 0.157$  and is the conversion value used in the “best-fit” limits. However, there is uncertainty between experimental measurements and the model at low recoil energies [7], and so the published analysis considers values of  $k$  from 0.1–0.2 with a uniform prior, i.e. each realization uniformly samples this range and uses the resulting  $k$  value in the conversion to  $\text{keV}_{\text{nr}}$ . In either case, the energy-scale conversion is accomplished by comparing Eq. 1 for an ER and NR with the same  $E_t$  giving

$$E_{\text{r,nr}} = E_{\text{r,ee}} \left( \frac{1 + eV_b/\epsilon_\gamma}{1 + Y(E_{\text{r,nr}})eV_b/\epsilon_\gamma} \right), \quad (3)$$

where  $E_{\text{r,ee}}$  and  $E_{\text{r,nr}}$  are the recoil energies calibrated to  $\text{keV}_{\text{ee}}$  and  $\text{keV}_{\text{nr}}$  respectively. The above equation is solved for  $E_{\text{r,nr}}$ , noting the dependence of  $Y(E_{\text{r,nr}})$ , for any given  $E_{\text{r,ee}}$ .

## 2 Description the Data

Ten text (`.txt`) files accompany this data release and can be found in the `data_files` directory of the accompanying `.zip` file. The names and descriptions of these files are

- **eventEnergy\_keVee.txt**: This file contains a single column of event energies, in units of  $\text{keV}_{\text{ee}}$ , and sorted by increasing energy. These 318 events are those from the final CDMSlite Run 2 spectrum used to compute WIMP-search limits. The energy range used in the WIMP-search results is defined to include all events between 56  $\text{eV}_{\text{ee}}$  and 2  $\text{keV}_{\text{ee}}$ . The spectrum generated by the events in this file is given in Fig. 1. The spectrum can be reproduced by using 10  $\text{eV}_{\text{ee}}$  sized bins with the lowest energy bin spanning 0–10  $\text{eV}_{\text{ee}}$ .
- **efficiency\_bestFit\_keVee.txt**: This file contains the “best-fit” WIMP-search efficiency below 2  $\text{keV}_{\text{ee}}$ . This curve and its uncertainty are the central-value efficiency and error bars representative of the central 68 % uncertainty interval ( $1\sigma$  equivalent). The file consists of four tab-separated columns, with the first column giving bin locations in  $\text{keV}_{\text{ee}}$ , the second column the total efficiency at that bin location, and the third/fourth column the lower/upper  $1\sigma$  uncertainty at each bin location. The uncertainties are given as the difference from the best-fit. The best-fit efficiency is given by the solid red curve in Fig. 2 while the  $1\sigma$  uncertainties are given by the dark red dotted envelope.

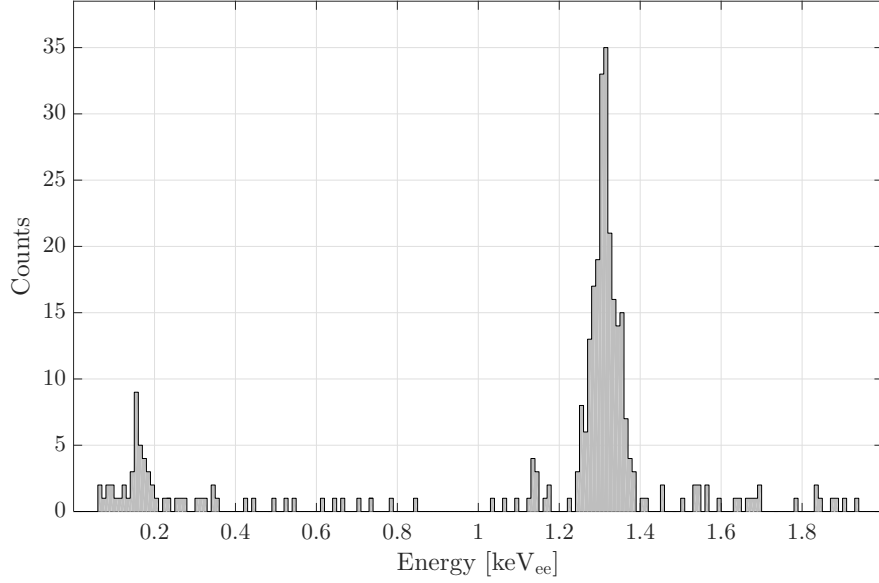

Figure 1: Energy spectrum of the CDMSlite Run 2 data between 56 eV<sub>ee</sub> and 2 keV<sub>ee</sub> as used in the official results.

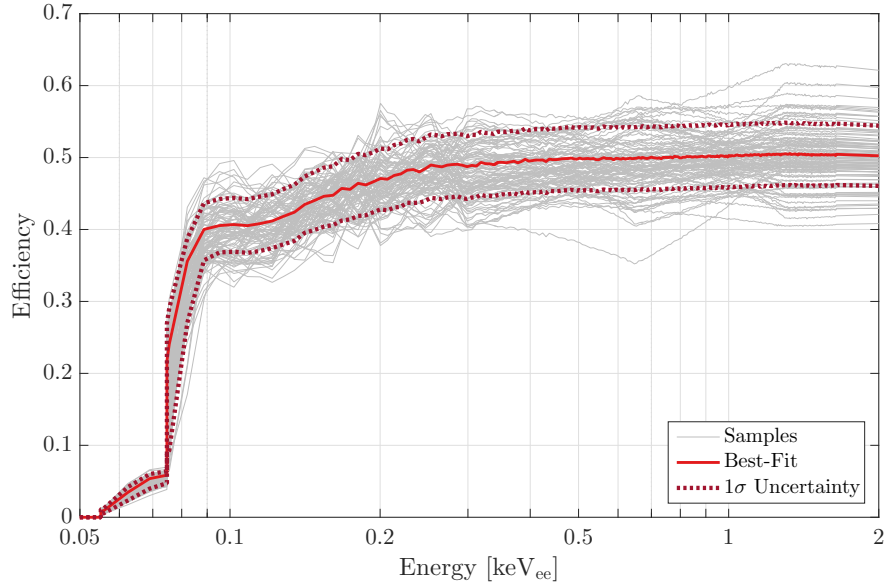

Figure 2: WIMP-search efficiency for CDMSlite Run 2 between 56 eV<sub>ee</sub> and 2 keV<sub>ee</sub> as used in the official results. The solid red curve is the “best-fit” efficiency with  $\pm 1\sigma$  uncertainty indicated by the dark red dotted envelope. 100 curves sampled from the underlying uncertainty distributions are shown in light gray.

- `efficiency_samples.txt`: As discussed above, the published analysis uses 1000 realizations of the analysis. This file contains 1000 realizations of the efficiency found by sampling the underlying uncertainty distributions used for computing the efficiency. For each of the 1000 realizations, a different sampled efficiency curve should be used. The file format is 1000 tab-separated columns, with each column being a different efficiency sample. The bins of every sample are the same as the bins given in `efficiency_bestFit.txt`. The first 100 of these samples are given by the light gray curves in Fig. 2.
- `limits_SI_GeVc2_cm2.txt`: This file contains the published spin-independent limit, with uncertainties, from the published analysis along with a best-fit limit. The file contains five tab-separated columns. The first column contains WIMP-masses in units of  $\text{GeV}/c^2$ . The remaining four columns contain limit values in units of  $\text{cm}^2$ . The second column is the best-fit limit, the third column is the official median limit, and the fourth/fifth column is the lower/upper bound on the 95 % uncertainty region of the official limit. These limits are shown in Fig. 3. The difference between how these limits are computed are given in Sec. 3. values of “Inf” in the files indicate that the given limit has no sensitivity at that particular WIMP mass.
- `limits_SD_*_GeVc2_cm2.txt`: These two files contain the published proton-/neutron-only ( $=p,n$  respectively) spin-dependent limits, with uncertainties, from the published analysis along with the corresponding best-fit limits. The format of the files is identical to that of the spin-independent limit file above and they are again shown in Fig. 3.
- `limits_SD_apan_*GeVc2.txt`: These four files contain the published mixed-coupling spin-dependent limits, with uncertainties, from the published analysis along with the corresponding best-fit limits. The analysis computes these limits on the dimensionless spin-dependent coupling constants  $a_p$  and  $a_n$  for WIMP masses of  $=2, 5, 10$ , and  $20 \text{ GeV}/c^2$ . The limits in this plane are presented in polar coordinates such that  $a_p = a \sin \theta$  and  $a_n = a \cos \theta$ . In each file, there are five tab-separated columns with the first containing angles  $\theta$  (in radians). The second column contains the radii  $a$  for the best-fit limit, the third is the official median limit, and the fourth/fifth column is the lower/upper bounds on the 95 % uncertainty region of the official limit. Each of these limits are given in Fig. 4.

### 3 Calculating the WIMP-Search Limits

In order to compute WIMP-search limits, four pieces are needed: the observed spectrum in  $\text{keV}_{\text{nr}}$ , the efficiency and exposure, a WIMP-signal model, and a limit-setting technique. This section describes how each of these items are used in the CDMSlite analysis in order to allow for reproduction of the WIMP interaction limits given in Refs. [1] (spin-independent) and [2] (spin-dependent).

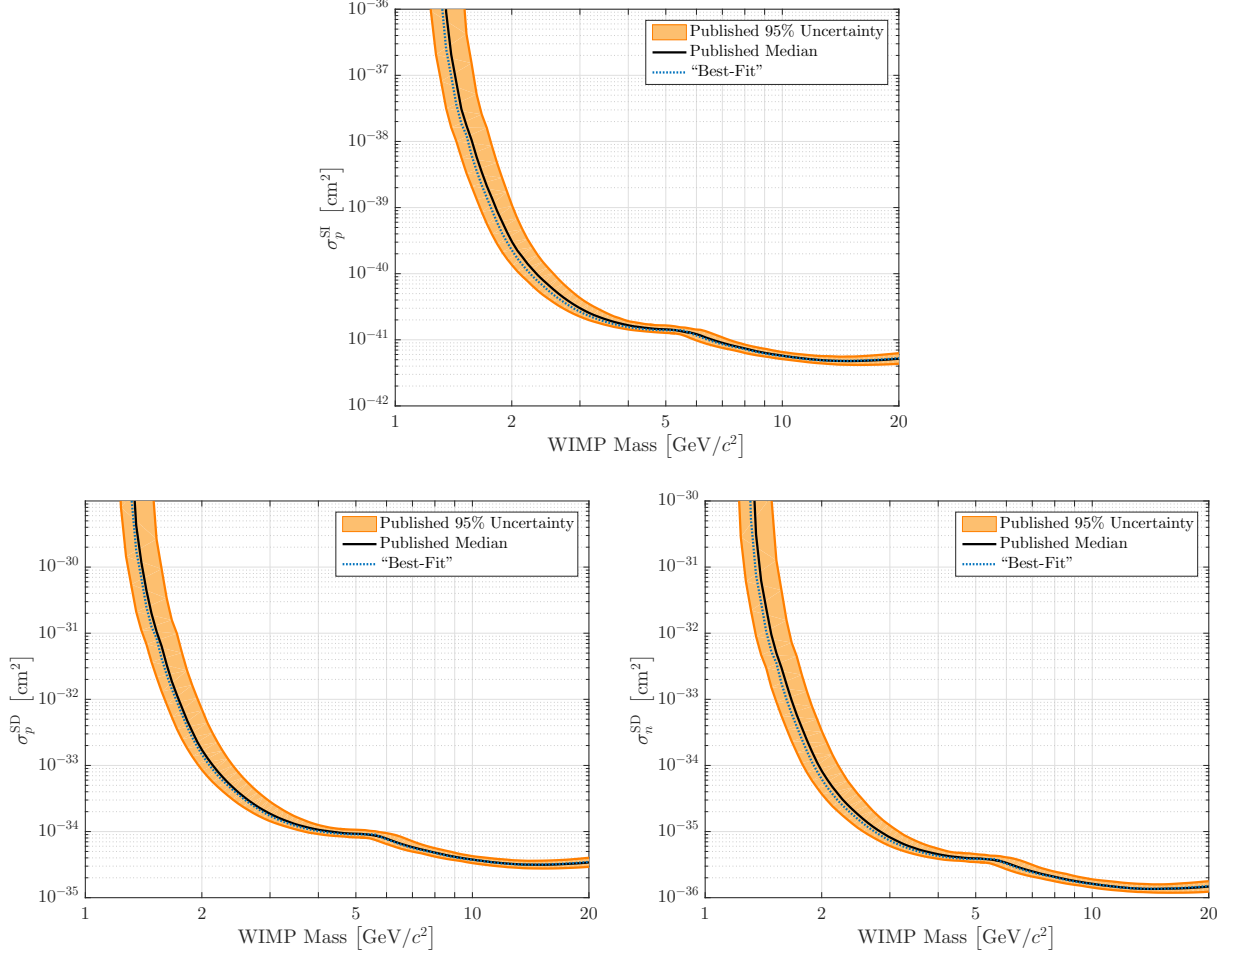

Figure 3: CDMSlite Run 2 WIMP-nucleon cross section 90 % confidence level upper limit computed using either the best-fit (blue dot) or official (black solid surrounded by orange band) efficiency and energy-scale conversions. Limits are placed on the spin-independent  $\sigma_p^{\text{SI}}$  (top), proton-only spin-dependent  $\sigma_p^{\text{SD}}$  (left), and neutron-only spin-dependent  $\sigma_n^{\text{SD}}$  (right) interactions.

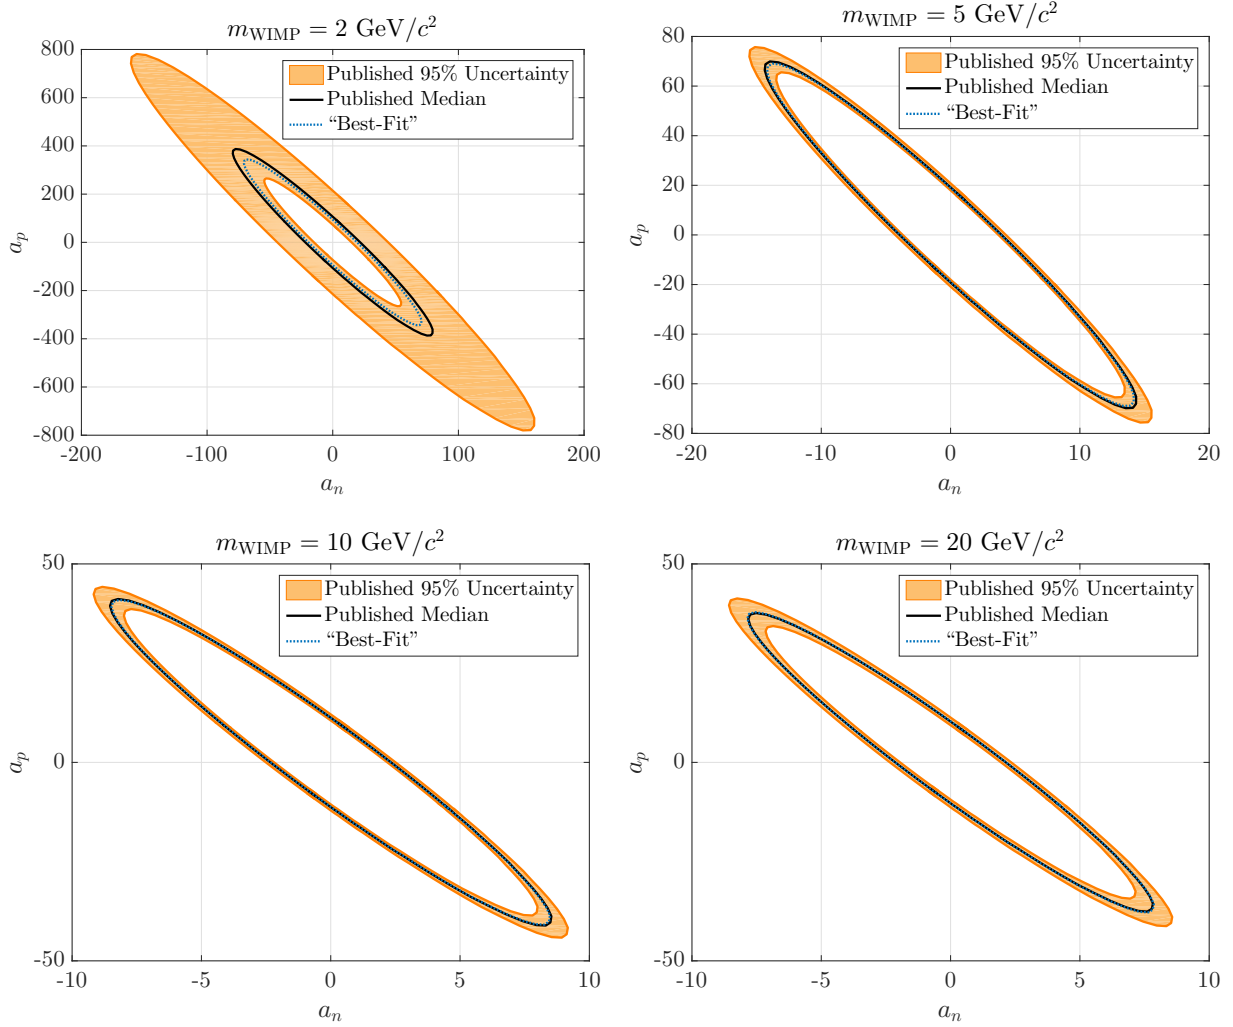

Figure 4: CDMSlite Run 2 90 % confidence level upper limits computed using either the best-fit (blue dot) or official (black solid surrounded by orange band) efficiency and energy-scale conversions on the spin-dependent WIMP-proton/-neutron coupling constants  $a_{p/n}$ . Limits are placed for WIMP masses of  $m_{\text{WIMP}} = 2$  (top left), 5 (top right), 10 (bottom left), and 20 (bottom right)  $\text{GeV}/c^2$  respectively.

### 3.1 Experimental Inputs

The CDMSlite Run 2 experimental inputs are the observed spectrum, signal efficiency, and total exposure. These are specified as follows.

**Observed Spectrum:** The observed energy spectrum is that given in `eventEnergy.txt` in  $\text{keV}_{\text{ee}}$ . The conversion to  $\text{keV}_{\text{nr}}$  performed in the published analysis is described in Sec. 1. For the best-fit limit, the standard Lindhard  $k = 0.157$  for Ge is used in the conversion. For the official limit, a  $k$  value is randomly and uniformly chosen between 0.1–0.2 for each sampled realization.

**Efficiency and Exposure:** The exposure of the CDMSlite Run 2 analysis is 70.10 kg d.  $^{73}\text{Ge}$  is the only odd-nucleon naturally found in Ge with an abundance of 7.76%. Thus, for spin-dependent calculations, the exposure should be reduced to this amount of the total at 5.44 kg d. For the best-fit limit, the efficiency curve from `efficiency_bestFit.txt` is used. For the official limit, the curves from `efficiency_samples.txt` are used. In either case, the bins must be converted to  $\text{keV}_{\text{nr}}$  and this is done in the same manner as the spectrum. For each sample used in computing the official limit, the same  $k$  value should be used for both the spectrum and efficiency conversions.

### 3.2 WIMP Signal Model

The published analysis uses the expected WIMP recoil rate in the detector as generally derived in Ref. [8] and summarized here.

**Halo Model:** The WIMP halo is assumed to be an isotropic, isothermal, and non-rotating sphere with a Maxwellian velocity distribution  $f(\mathbf{v}, \mathbf{v}_{\text{E}})$  of the form

$$f(\mathbf{v}, \mathbf{v}_{\text{E}}) \propto \rho_0 e^{-|\mathbf{v} + \mathbf{v}_{\text{E}}|^2/v_0^2}, \quad (4)$$

where  $\mathbf{v}$  is the WIMP velocity,  $v_0 = 220 \text{ km s}^{-1}$  is the most probable WIMP velocity in the halo, and  $v_{\text{E}} = |\mathbf{v}_{\text{E}}| = 232 \text{ km s}^{-1}$  is the mean circular velocity of the Earth through the halo (ignoring the Earth’s orbit around the Sun). The other astrophysical assumptions used are a local dark matter density of  $\rho_0 = 0.3 \text{ GeV c}^{-2} \text{ cm}^{-3}$  and a Galactic escape velocity of  $v_{\text{esc}} = 544 \text{ km s}^{-1}$ . The uncertainties in these astrophysical parameters are considered in [2] and are not discussed here. Note that the integration over the velocity distribution function in Ref. [8] allows for non-physical negative rates for certain velocity combinations. Equation 3.13 of Ref. [8], the differential rate in terms of the target’s recoil energy  $E_{\text{r}}$ , is replaced with the more complete result (see e.g. Appendix A of Ref. [9]) of

$$\frac{dR}{dE_{\text{r}}} = \frac{R_0}{E_0 r} \frac{k_0}{k_1} \frac{\sqrt{\pi}}{4y} \begin{cases} \text{erf}(x+y) - \text{erf}(x-y) - \frac{4}{\sqrt{\pi}} y e^{-z^2} & 0 < x < z-y \\ \text{erf}(z) - \text{erf}(x-y) - \frac{2}{\sqrt{\pi}} (y+z-x) e^{-z^2} & z-y < x < z+y \\ 0 & y+z < x, \end{cases} \quad (5)$$

where  $R_0$  and  $r$  are the total rate and kinematic factors defined in Ref. [8],  $k_0$  and  $k_1$  are normalization factors which are also defined in Ref. [8],  $E_0 = (1/2) m_\chi v_0^2$  with  $m_\chi$  as the mass of the WIMP,  $x = v_{\min}/v_0$ ,  $y = v_E/v_0$ , and  $z = v_{\text{esc}}/v_0$ . The minimum velocity for a WIMP to impart  $E_r$  on a target of mass  $m_T$  is  $v_{\min} = \sqrt{m_T E_r / 2\mu_T^2}$ , using the WIMP-target reduced mass of  $\mu_T = m_T m_\chi / (m_T + m_\chi)$ . The value of  $R_0$  uses the atomic mass number  $A = 72.64$  for Ge and  $A = 73$  for the spin-interaction sensitive  $^{73}\text{Ge}$

**Nuclear Form Factor:** In Ref. [8], the WIMP-nucleus cross section is generally taken to be of the form

$$\sigma(q) = \sigma^{\text{SI}}(q) + \sigma^{\text{SD}}(q) = \sigma_0^{\text{SI}} F_{\text{SI}}^2(q) + \sigma_0^{\text{SD}} F_{\text{SD}}^2(q), \quad (6)$$

where  $q$  is the momentum transferred in the collision and the spin-independent (SI) and spin-dependent (SD) contributions are each separated into the total zero-momentum cross section  $\sigma_0^{\text{SI/D}}$  and the nuclear form factor  $F_{\text{SI/D}}$ . The different spin-dependencies are treated separately below

**Spin Independent:** The Helm expression is used for the spin-independent nuclear form factor [10]

$$F_{\text{SI}}(q) = 3 \frac{j_1(qr_n)}{qr_n} e^{-\frac{1}{2}(qs)^2}, \quad (7)$$

where  $j_1(qr_n)$  is the spherical Bessel function of the first order and  $q$  is the momentum transferred to the nucleus in the scatter. For the remaining parameters, the parameterization preferred in Ref. [8] is used which gives  $r_n^2 = c^2 + (7/3) \pi^2 a^2 - 5s^2$ ,  $c \simeq 1.23A^{1/3} - 0.6$  fm,  $s \simeq 0.9$  fm, and  $a \simeq 0.52$  fm, with  $A$  as the atomic mass number.

**Spin Dependent:** The spin-dependent nuclear form factor is defined in reference to the nuclear spin-structure function  $S_T(q)$  as

$$F_{\text{SD}}^2(q) \equiv S_T(q)/S_T(0). \quad (8)$$

The spin-structure function is given by a linear combination of isoscalar  $S_{00}(q)$ , isovector  $S_{11}(q)$ , and interference  $S_{01}(q)$  terms as

$$S_T(q) = a_0^2 S_{00}(q) + a_1^2 S_{11}(q) + a_0 a_1 S_{01}(q). \quad (9)$$

The isoscalar  $a_0$  and isovector  $a_1$  coupling constants are related to the proton  $a_p$  and neutron  $a_n$  coupling constants as  $a_0 = a_p + a_n$  and  $a_1 = a_p - a_n$ . The proton- and neutron-only models are defined as  $a_1 = a_0 = 1$  (i.e.  $a_p = 1$ ,  $a_n = 0$ ) and  $a_1 = -a_0 = 1$  (i.e.  $a_p = 0$ ,  $a_n = 1$ ). In these models, the structure function reduces to

$$S_T^p(q) = a_p^2 (S_{00}(q) + S_{11}(q) + S_{01}(q)) \equiv a_p^2 S_p(q) \quad (10)$$

$$S_T^n(q) = a_n^2 (S_{00}(q) + S_{11}(q) - S_{01}(q)) \equiv a_n^2 S_n(q). \quad (11)$$



The Run 2 analysis uses the structure function calculation for  $^{73}\text{Ge}$  from Klos *et al.* [11]. These authors fit ninth-degree polynomials to the upper and lower uncertainty bands from their calculations as functions of a dimensionless momentum variable which is nuclei dependent. Although not in the published manuscript, the coefficients for these polynomials can be found in the Appendix D of their arXiv preprint [arXiv:1304.7684](https://arxiv.org/abs/1304.7684). Polynomial coefficients are given for each of  $S_{00}(q)$ ,  $S_{11}(q)$ ,  $S_{01}(q)$ ,  $S_p(q)$ , and  $S_n(q)$ . For limits computed in the proton-/neutron only models, these latter functions are directly used, while, for any other coupling-constant combination, the isoscalar/isovector functions are used. In any case, both the minimum and maximum fit functions are computed and their average taken as the final structure function.

**Normalization:** The CDMSlite analysis follow the standard practice of presenting limits on the momentum-independent WIMP-nucleon cross sections. Scaling limits on the WIMP-nucleus cross sections,  $\sigma_0^{\text{SI/D}}$  in Eq. 6, to a limit on the interaction of a WIMP and a single nucleon is accomplished differently for different spin dependencies as discussed next.

**Spin Independent:** The spin-independent interaction is assumed to be isoscalar with the WIMP-proton coupling  $f_p$ . The standard zero-momentum spin-independent cross section for a WIMP to scatter off any target nucleus can then be written as

$$\sigma_0^{\text{SI}} = \frac{4\mu_T^2}{\pi} A^2 f_p^2. \quad (12)$$

The WIMP-nucleus cross section is then scaled to the WIMP-nucleon cross section as

$$\sigma_0^{\text{SI}} = \left( \frac{\mu_T}{\mu_p} A \right)^2 \sigma_p^{\text{SI}}, \quad (13)$$

where  $\mu_p$  is the reduced mass of the WIMP-nucleon system (the difference between the proton and neutron mass are neglected) and  $\sigma_p^{\text{SI}}$  is the cross section for single-nucleon WIMP interaction. The momentum-dependent cross section is then the combination of Eqs. 7 and 13

$$\sigma^{\text{SI}}(q) = \sigma_0^{\text{SI}} \cdot F_{\text{SI}}^2(q) \quad (14)$$

$$= \left( \frac{\mu_T}{\mu_p} A \right)^2 \sigma_p^{\text{SI}} \cdot \left( 3 \frac{j_1(qr_n)}{qr_n} \right)^2 e^{-(qs)^2}, \quad (15)$$

with the form factor parameters described above.

**Proton-/Neutron-only Spin Dependent:** The standard zero-momentum spin-dependent cross section for a WIMP to scatter of any target nucleus, of nuclear spin  $J$  ( $J = 9/2$  for  $^{73}\text{Ge}$ ), is

$$\sigma_0^{\text{SD}} = \frac{32}{2J+1} G_F^2 \mu_T^2 S_T(0), \quad (16)$$

where  $G_F$  is Fermi's constant. An analytical expression for  $S_T(0)$  is given in Ref. [11] which evaluates to  $3a_{p/n}^2/2\pi$  for a free proton/neutron with  $J = 1/2$ .

The WIMP-nucleus cross section is then scaled to the WIMP-proton/-neutron cross section as

$$\sigma_0^{\text{SD}} = \frac{4\pi}{3} \frac{1}{(2J+1)} \left( \frac{\mu_T}{\mu_{p/n}} \right)^2 \frac{S_T(0)}{a_{p/n}^2} \sigma_{p/n}^{\text{SD}}, \quad (17)$$

where  $\sigma_{p/n}^{\text{SD}}$  is the WIMP-nucleon cross section for a free proton/neutron. The momentum-dependent cross section is then the combination of Eqs. 8 and 17

$$\sigma^{\text{SD}}(q) = \sigma_0^{\text{SD}} \cdot F_{\text{SD}}^2(q) \quad (18)$$

$$= \frac{4\pi}{3} \frac{1}{(2J+1)} \left( \frac{\mu_T}{\mu_{p/n}} \right)^2 \frac{S_T(0)}{a_{p/n}^2} \sigma_{p/n}^{\text{SD}} \cdot \frac{S_T(q)}{S_T(0)} \quad (19)$$

$$= \frac{4\pi}{3} \frac{1}{(2J+1)} \left( \frac{\mu_T}{\mu_{p/n}} \right)^2 \frac{\sigma_{p/n}^{\text{SD}}}{a_{p/n}^2} S_T(q). \quad (20)$$

Limits are then computed on the  $\sigma_p^{\text{SD}}$  for the proton-only model and  $\sigma_n^{\text{SD}}$  for the neutron-only model after appropriately evaluating  $S_T(q)$  for  $^{73}\text{Ge}$  and the specific model as discussed above.

**Mixed-Coupling Spin Dependent:** Limits are also set, for a given WIMP mass, jointly on the spin-dependent WIMP-proton and -neutron coupling constants. For these limits, the normalization is from the WIMP-nucleus cross section to the WIMP-nucleon coupling constants. These limits are computed by writing the coupling constants in polar coordinates such that  $a_p = a \sin \theta$  and  $a_n = a \cos \theta$ . Using this coordinate system, Eq. 9 is written as

$$S_T(q) = a^2 [(1 + \sin 2\theta) S_{00}(q) - \cos 2\theta S_{10}(q) + (1 - 2 \sin \theta \cos \theta) S_{11}(q)] \quad (21)$$

$$\equiv a^2 f(q; \theta). \quad (22)$$

Using this expression when combining Eqs. 8 and 16 gives

$$\sigma^{\text{SD}}(q) = \sigma_0^{\text{SD}} \cdot F_{\text{SD}}^2(q) \quad (23)$$

$$= \frac{32}{2J+1} G_{\text{F}}^2 \mu_T^2 a^2 f(q; \theta). \quad (24)$$

For a any given  $\theta$ , limits are then computed on  $a^2$  and the results computed on  $a_p$ - $a_n$  by converting back to the Cartesian coordinate system.

### 3.3 Limit-Setting Technique

The user is free to use any desired statistical method for computing upper limits. The published analysis uses the high-statistics extension of the Optimum Interval (OI) method, as described in Ref. [12], to set limits on the cross section for WIMP masses from 1-20 GeV/ $c^2$ . Using the “best-fit” efficiency and energy-scale conversion will result in a single curve, such as the blue dotted curves in Figs. 3 and 4. To compute the official results, a limit curve is computed for each of the 1000 efficiency curves using 1000 different energy-scale conversions

with the median and 2.5<sup>th</sup> and 97.5<sup>th</sup> percentiles defining the solid black curves surrounded by orange band in Figs. 3 and 4.

The OI code is publicly available for download from Ref. [13], which includes documentation on the individual-script level. For convenience, a stand-alone implementation of the code for these data is provided in the `OI_code` directory of the release. The OI code is written in FORTRAN with the primary function being in `lite2Upper.f`. The code has been compiled for a Unix operating system, resulting in the `lite2Upper` executable. It can be recompiled on a Unix system using

```
gfortran -frecord-marker=4 -o lite2Upper lite2Upper.f UpperLimNew2.f
y_vs_CLf2.f CMaxinfNew2.f ConfLev2.f ConfLevNew2.f Cinf2.f CERN_Stuff2.f
```

or

```
f77 -o lite2Upper lite2Upper.f UpperLimNew2.f y_vs_CLf2.f CMaxinfNew2.f
ConfLev2.f ConfLevNew2.f Cinf2.f CERN_Stuff2.f
```

The `ULinput` file is the input file read which is hard-coded to be ready by the FORTRAN code. The provided `ULinput` file contains the appropriately formatted spectrum and efficiency information from these data for the spin-independent “best-fit” limit parameters. See the documentation of the public code at Ref. [13] for further details with regards to properly formatting the input. The FORTRAN code produces an output file `ULoutput`, the first two columns of which are the SI WIMP-nucleon cross section limit ( $\text{cm}^2$ ) and WIMP mass ( $\text{GeV}/c^2$ ) respectively. The provided `ULoutput` matches the provided `ULinput`, and gives the “best-fit” SI limit.

## References

- [1] R. Agnese *et al.*, “New Results from the Search for Low-Mass Weakly Interacting Massive Particles with the CDMS Low Ionization Threshold Experiment,” *Phys. Rev. Lett.* **116**, 071301 (2016).
- [2] R. Agnese *et al.*, “Low-Mass Dark Matter Search with CDMSlite,” *Phys. Rev. D* **97**, 022002 (2018).
- [3] B. Neganov and V. Trofimov, “Calorimetric method measuring ionizing radiation,” *Otkrytia i Izobret.* **146**, 215 (1985).
- [4] P. N. Luke, “Voltage-assisted calorimetric ionization detector,” *J. Appl. Phys.* **64**, 6858 (1988).
- [5] F. E. Emery and T. A. Rabson, “Average Energy Expended Per Ionized Electron-Hole Pair in Silicon and Germanium as a Function of Temperature,” *Phys. Rev.* **140**, A2089–A2093 (1965); R. Pehl, F. Goulding, D. Landis, and M. Lenzlinger, “Accurate determination of the ionization energy in semiconductor detectors,” *Nucl. Instrum. Methods* **59**, 45–55 (1968).

- [6] J. Lindhard, V. Nielsen, M. Scharff, and P. V. Thomsen, “Integral Equations Governing Radiation Effects (Notes On Atomic Collisions III ),” *Mat. Fys. Medd. Dan. Vid. Selsk.* **33** (1963); J. Lindhard, M. Scharff, and H. E. Schiott, “Range Concepts And Heavy Ion Ranges (Notes On Atomic Collisions II ),” *Mat. Fys. Medd. Dan. Vid. Selsk.* **33** (1963); J. Lindhard, V. Nielsen, and M. Scharff, “Approximation Method In Classical Scattering By Screened Coulomb Fields (Notes on Atomic Collisions, I),” *Mat. Fys. Medd. Dan. Vid. Selsk.* **36** (1968).
- [7] D. Barker and D.-M. Mei, “Germanium detector response to nuclear recoils in searching for dark matter,” *Astropart. Phys.* **38**, 1–6 (2012).
- [8] J. Lewin and P. Smith, “Review of mathematics, numerical factors, and corrections for dark matter experiments based on elastic nuclear recoil,” *Astropart. Phys.* **6**, 87–112 (1996).
- [9] F. Donato, N. Fornengo, and S. Scopel, “Effects of galactic dark halo rotation on WIMP direct detection,” *Astropart. Phys.* **9**, 247–260 (1998).
- [10] R. H. Helm, “Inelastic and Elastic Scattering of 187-Mev Electrons from Selected Even-Even Nuclei,” *Phys. Rev.* **104**, 1466–1475 (1956).
- [11] P. Klos, J. Menéndez, D. Gazit, and A. Schwenk, “Large-scale nuclear structure calculations for spin-dependent WIMP scattering with chiral effective field theory currents,” *Phys. Rev. D* **88**, 083516 (2013).
- [12] S. Yellin, “Extending the optimum interval method,” [arXiv:0709.2701](https://arxiv.org/abs/0709.2701) .
- [13] S. Yellin, “<http://titus.stanford.edu/Upperlimit/>,” (2015).
